# Supplementary material for: Reach-Avoid Analysis for Polynomial Stochastic Differential Equations
Source: arXiv:2208.10752 source file (2023-12-21)
Supplement: Supplementary file 1 [file Appendix.tex]

\section*{Appendix}
The proof of Lemma \ref{eq}:
\begin{proof}
We first prove that \[\mathbb{P}(\widehat{\bm{X}}^{\bm{x}_0}(t,\bm{w})\in \mathcal{T})=\mathbb{P}(\widehat{\tau}_{\mathcal{T}}^{\bm{x}_0}(\bm{w})\leq t)\] with $t\geq 0$.

Let $A_t=\{\bm{w}\in \Omega \mid \widehat{\bm{X}}^{\bm{x}_0}(t,\bm{w})\in \mathcal{T}\}$ and $B_t=\{\bm{w}\in \Omega\mid \widehat{\tau}_{\mathcal{T}}^{\bm{x}_0}(\bm{w})\leq t\}.$ If $A_t=B_t$, \[\mathbb{P}(A_t)=\mathbb{P}(B_t)\] holds. 
We just need to prove that $A_t=B_t$. 

Obviously, if $\bm{w}\in A_t$, we have that \[\widehat{\bm{X}}^{\bm{x}_0}(t,\bm{w})\in \mathcal{T}\] and \[\widehat{\bm{X}}^{\bm{x}_0}(\tau,\bm{w})\in \mathcal{X}, \forall \tau\in [0,t].\] Thus, $\widehat{\tau}_{\mathcal{T}}^{\bm{x}_0}(\bm{w})\leq t$, implying that \[\bm{w}\in B_t.\] Consequently, $A_t\subseteq B_t$.

If $\bm{w}\in B_t$,  $\widehat{\tau}_{\mathcal{T}}^{\bm{x}_0}(\bm{w})\leq t$ and thus \[\widehat{\bm{X}}^{\bm{x}_0}(t,\bm{w}) \in \mathcal{T}.\] Therefore, $\bm{w}\in A_t$ and thus $B_t\subseteq A_t$. 

Consequently,  $A_t=B_t$ and thus \[\mathbb{P}(A_t)=\mathbb{P}(B_t).\] 

    Also, since \[A_{\tau_2}\subseteq A_{\tau_1}\] and \[B_{\tau_2}\subseteq B_{\tau_1}\] for $0\leq \tau_2\leq \tau_1$, according to the Monotone Convergence Theorem for measurable sets (e.g.,Theorem 2.16 in \cite{yeh2006real}) we have \[\lim_{t\rightarrow \infty}\mathbb{P}(\widehat{\bm{X}}^{\bm{x}_0}(t,\bm{w})\in \mathcal{T})=\mathbb{P}(\widehat{\tau}_{\mathcal{T}}^{\bm{x}_0}(\bm{w})<\infty).\]
The proof is completed.
\end{proof}

\oomit{
In this section we give a formal proof of the statement in Remark \ref{determi}. %Before this we give formal presentation of these statements below. 
\begin{corollary}
If there exist $v(\bm{x})\in \mathcal{C}^1(\widehat{\mathcal{X}})$ and $w(\bm{x})\in \mathcal{C}^1(\widehat{\mathcal{X}})$ satisfying \eqref{upper3}, where \[\mathcal{A}v(\bm{x})=\frac{\partial v}{\partial \bm{x}}\bm{b}(\bm{x})\] and \[\mathcal{A}u(\bm{x})=\frac{\partial u}{\partial \bm{x}}\bm{b}(\bm{x})\] 
for $\bm{x}\in \mathcal{X}\setminus \mathcal{T}$, then 
\[\{\bm{x}\in \widehat{\mathcal{X}}\mid v(\bm{x})>0\} \subset {\rm RA},\] where ${\rm RA}$ is the reach-avoid set in \eqref{deter_reach}.
\end{corollary}
\begin{proof}
Let $\bm{x}_0\in \{\bm{x}\in \widehat{\mathcal{X}}\mid v(\bm{x})>0\}$. If $\bm{x}_0\in {\rm RA}$, it is clear that the conclusion holds. Thus, we only consider 
\[\bm{x}_0\in \{\bm{x}\in \widehat{\mathcal{X}}\mid v(\bm{x})>0\}\setminus {\rm RA}.\]

The constraint that $v(\bm{x})\leq 0$ for $\bm{x}\in \widehat{\mathcal{X}}\setminus \mathcal{X}$ indicates that \[\bm{x}_0\in \mathcal{X}\setminus {\rm RA}.\]

Therefore, there exist three cases for the trajectory $\bm{X}^{\bm{x}_0}(\cdot): \mathbb{R}_{\geq 0} \rightarrow \mathbb{R}^n$:
\begin{enumerate}
    \item there exists $t\in \mathbb{R}_{\geq 0}$ such that \[[\forall {\tau \in [0,t)}. \bm{X}^{\bm{x}_0}(\tau)\in \mathcal{X}\setminus \mathcal{T}] \bigwedge [\bm{X}^{\bm{x}_0}(t)\in \widehat{\mathcal{X}}\setminus \mathcal{X}].\]
    \item $\bm{X}^{\bm{x}_0}(t)\in \mathcal{X}\setminus \mathcal{T}$ for $t\in \mathbb{R}_{\geq 0}$.
    \item there exists $t\in \mathbb{R}_{\geq 0}$ such that \[[\forall {\tau \in [0,t)}. \bm{X}^{\bm{x}_0}(\tau)\in \mathcal{X}\setminus \mathcal{T}] \bigwedge [\bm{X}^{\bm{x}_0}(t)\in  \mathcal{T}].\]
\end{enumerate}

We first prove that the first case does not hold. Assume that it holds. Then according to constraint \[\mathcal{A}v(\bm{x})\geq 0, \forall \bm{x}\in \mathcal{X}\setminus \mathcal{T},\] we have that 
\begin{equation}
    \label{larger}
v(\bm{X}^{\bm{x}_0}(t))\geq v(\bm{x}_0)>0.
\end{equation}
However, since $v(\bm{x})\leq 0$ for $\bm{x}\in \widehat{\mathcal{X}}\setminus \mathcal{X}$ and $\bm{X}^{\bm{x}_0}(t)\in \widehat{\mathcal{X}}\setminus \mathcal{X}$, $v(\bm{X}^{\bm{x}_0}(t))\leq 0$. This contradicts \eqref{larger}. Thus, the first case does not hold.

Next, we prove that the second case does not hold either. Assume that $\bm{X}^{\bm{x}_0}(t)\in \mathcal{X}\setminus \mathcal{T}$ for $t\in \mathbb{R}_{\geq 0}$. According to the constraint $-v(\bm{x})+\mathcal{A}u(\bm{x})\geq 0$ for $\bm{x}\in \mathcal{X}\setminus \mathcal{T}$, we have that 
\[-\int_{0}^{t}v(\bm{X}^{\bm{x}_0}(\tau)) d\tau +\int_{0}^t \mathcal{A}u(\bm{X}^{\bm{x}_0}(\tau)) d\tau \geq 0,\]
indicating that 
\[u(\bm{X}^{\bm{x}_0}(t))-u(\bm{x}_0)\geq \int_{0}^{t}v(\bm{X}^{\bm{x}_0}(\tau)) d\tau.\]
Also, since $\mathcal{A}v(\bm{x}) \geq 0$ for $\bm{x}\in \mathcal{X}\setminus \mathcal{T}$, we have that 
\[u(\bm{X}^{\bm{x}_0}(t))-u(\bm{x}_0)\geq t v(\bm{x}_0).\]
By letting $t\rightarrow 0$, we have that 
$v(\bm{x}_0)\leq 0$, which contradicts $v(\bm{x}_0)>0$. Thus, the second case does not hold either. 

Therefore, the third case holds and thus $\bm{x}_0\in RA$, implying that 
\[\{\bm{x}\in \widehat{\mathcal{X}}\mid v(\bm{x})>0\} \subset {\rm RA}.\]
\end{proof}
}
